# Supplementary material for: DreamWaQ++: Obstacle-Aware Quadrupedal Locomotion With Resilient Multi-Modal Reinforcement Learning
Source: arXiv:2409.19709 source file (2026-02-26)
Supplement: Supplementary file 1 [file supplementaries.tex]

\section{Supplementaries}\label{section:supp}

\begingroup
% \renewcommand{\thesubsection}{S\arabic{subsection}}

% \renewcommand{\figurename}{Fig.}
% \renewcommand{\thefigure}{S\arabic{figure}}
% \captionsetup[figure]{labelfont=bf,labelsep=period,font=normalsize}

% \renewcommand{\thetable}{S\arabic{table}}
% \captionsetup[table]{labelfont=bf,labelsep=period,font=normalsize}

% \setcounter{figure}{0}

\subsection{Nomenclature}\label{supp:nomenclature}
\begin{table}[h!]
    \small
    \begin{tabular}{ll}
        \textbf{Notations} \\
        $(\cdot)^\textbf{des}$ & Target or desired value\\
        $(\cdot)^\textbf{cmd}$ & Command value\\
        $\textbf{g}$ & Gravity vector projected on the robot's body frame\\
    \end{tabular}
\end{table}

\begin{table}[h!]
    \small
    \begin{tabular}{ll}
        \textbf{Operators} \\
        $\mathrm{exp(\cdot)}$ & Exponential function\\
        $\mathrm{var(\cdot)}$ & Variance function\\
         $\mathrm{\sigma(\cdot)}$ & Standard deviation function\\
    \end{tabular}
\end{table}

\begin{table}[H]
    \small
    \begin{tabular}{ll}
        \textbf{Abbreviations} \\
        IMU & Inertial measurement unit\\
        HAA & Hip abduction/adduction\\
        HFE & Hip flexion/extension\\
        KFE & Knee flexion/extension\\
        FR & Front right\\
        FL & Front left\\
        RR & Rear right\\
        RL & Rear left\\
        MLP & Multi-layer perceptron\\
        PaCMAP & Pairwise controlled manifold approximation projection\\
        PD & Proportional and derivative\\
        POMDP & Partially observable Markov decision process\\
        PPO & Proximal policy optimization\\
        t-SNE & t-distributed stochastic neighbor embedding\\
        VAE & Variational autoencoder\\
    \end{tabular}
\end{table}

\begin{table*}[h!]
    \centering
    \caption{\textbf{Summary of state-of-the-art algorithms}. \textit{Versatility} indicates whether the learned controller can be flexibly used for various tasks, e.g.~using a teleoperation or with a high-level planner. \textit{Computation} indicates the number of onboard processor(s) used on the robot to infer the whole locomotion controller, including the processor(s) used for preprocessing the exteroceptive measurement. \textit{Exteroception} indicates what type of exteroceptive measurement is required as an input.  \textit{Training stage} indicates the number of separate training procedures. Training stage~$\!=\!1$ means that there is no pre-training or fine-tuning of the networks using additional training instances. Training stage~$\!>\!1$ means additional training instances are required such as distillation, fine-tuning, and pre-training of some auxiliary modules.}
    \small
    \begin{tabular}{|c|c|c|c|c|c|} \hline 
         \multirow{2}{*}{Algorithm}&   \multirow{2}{*}{Robot}& \multicolumn{2}{|c|}{Deployment}&  \multirow{2}{*}{Exteroception}& Training\\ \cline{3-4}
         \multirow{2}{*}{} & \multirow{2}{*}{} &  Versatility&Computation& \multirow{2}{*}{}&stage\\\hline
         Miki \textit{et al}.~\cite{miki2022learning}&   ANYmal-C& \cmark&  1 (GPU)&Elevation map&  2\\ \hline 
         Agarwal \textit{et al}.~\cite{agarwal2022legged}&   Unitree A1& \xmark&  1&Depth image&  2\\ \hline 
         Yang \textit{et al}.~\cite{yang2023neural}&   Unitree A1& \xmark&  1& Depth image&  2\\ \hline 
         Hoeller \textit{et al}.~\cite{hoeller2023anymal}&   ANYmal-D& \cmark&  2& Surround pointcloud& 6\\ \hline 
		 Cheng \textit{et al}.~\cite{cheng2023parkour}&   Unitree A1& \cmark&  2& Depth image& 2\\ \hline 
         DreamWaQ++ (ours)&   Unitree Go1& \cmark&  1& Forward pointcloud&  1\\ \hline
    \end{tabular}
    
    \label{table:comparison}
\end{table*}

\subsection{Problem formulation}
We formulate the problem as a partially observable Markov decision process (POMDP) because, in the real world, the robot has no direct access to the exact state of the environment. We try to solve the problem by leveraging few shot meta--reinforcement learning (meta--RL) via task inference, which trains a separate network that can predict the task or context of the environment leveraging a few data points in conjunction with the policy network.

The environment is a POMDP defined by the tuple $\mathcal{M}=(\mathcal{S},\mathcal{O},\mathcal{A},d_0,p,r,\gamma)$. The full state, partial observation, and action are continuous, and defined by $\mathcal{\textbf{s}\in\mathcal{S}}$, $\mathcal{\textbf{o}\in\mathcal{O}}$, and $\mathcal{\textbf{a}\in\mathcal{A}}$, respectively. Generally, every environment with different physical properties, such as the robot's hardware, terrain properties, and commanded velocity, is categorized as a different POMDP sampled from a task distribution $P(\mathcal{M})$.

The environment starts with an initial state distribution, $d_0(\textbf{s}_0)$; progresses with a system dynamics $p(\textbf{s}_{t+1}|\textbf{s}_{t},\textbf{a}_{t})$; and obtains a reward, $r:\mathcal{S}\times\mathcal{A}\to\mathcal{R}$ for every action at a given state. The discount factor is defined by $\gamma\in[0,1)$. 

The goal of meta--RL in our problem setting is to learn a context encoder network, $\phi(\textbf{z}|\textbf{o},\textbf{a})$, that can infer the task in a form of a context vector, $\textbf{z}$, given available observations and actions. 
% In this paper, we define a temporal observation at time $t$ over the past $H$ measurements as $\textbf{o}^H_t=\begin{bmatrix}\textbf{o}_t & \textbf{o}_{t-1} \dots \textbf{o}_{t-H} \end{bmatrix}^T$. 

Prior works have enjoyed the benefit of task inference for fast adaptation of the learned control policy in the real world by explicitly training a context encoder that predicts some physical properties of the world, such as ground friction and restitution~\cite{kumar2021rma,lee2020learning,miki2022learning}. However, those works assumed that the contexts were available in training time. Although this relaxed assumption can facilitate learning, it also limits the solution space of the context. Moreover, as some context might not be directly identifiable from a short history of observations, the context encoder may fail to generate an informative context~\cite{xie2022robust}. 

In contrast, we trained a context encoder in an unsupervised manner. In DreamWaQ~\cite{nahrendra2023dreamwaq}, the context encoder is built upon the $\beta$--variational autoencoder ($\beta$--VAE) architecture that predicts the future observations. The advantages of leveraging $\beta$--VAE in DreamWaQ's framework are twofold. First, a higher degree of latent disentanglement induced by the $\beta$--VAE enables distinguishable task inference, which significantly helps learning and adaptation. Second, the stochastic network architecture makes the context encoder more robust to epistemic uncertainty when given out of distribution (OOD) observations.

In this work, the context encoder is trained jointly with a height reconstructor network to build a map using a stream of historical proprioceptive and exteroceptive data. This method is theoretically possible because it is built on the idea of simultaneous localization and mapping~(SLAM) where accumulated geometrical feature points along with odometry can be fused to build a map around the robot. More specifically, the context encoder in DreamWaQ++ consists of three attention mechanisms, i.e.~cross--modal, temporal, and spatial attentions.

% ===================================================================================
\begin{table}[t!]
% \begin{threeparttable} 
\centering
% \captionsetup{font=footnotesize, singlelinecheck=false}
\caption{\textbf{Hardware comparison}. The hardware parameters are obtained by measuring the official open-sourced 3D model of the corresponding robot~\cite{unitreea1,unitreego1}.}
\label{table:hardware_comparison}
\begin{center}
\begin{tabular}{lcc}
\hline \hline
Parameter           & Unitree A1~\cite{unitreea1} & Unitree Go1~\cite{unitreego1} \\ \hline 
Total weight (kg)       & $12$ & $13$      \\ 
Base length (m)         & $0.27$ & $0.38$      \\ 
Base width (m)          & $0.19$ & $0.19$      \\ 
Base height (m)         & $0.11$ & $0.11$      \\ 
Standing height (m)     & $0.4$ & $0.4$      \\ 
Thigh length (m)        & $0.2$ & $0.2$      \\ 
Calf length (m)         & $0.2$ & $0.2$      \\ 
Max. hip torque (Nm)    & $33.5$ & $23.7$      \\ 
Max. thigh torque (Nm)  & $33.5$ & $23.7$      \\ 
Max. calf torque (Nm)   & $33.5$ & $33.5$      \\

\hline \hline
\end{tabular}
\end{center}
\end{table}
% ===================================================================================

\subsection{Real-world Stair-climbing Race}\label{supp:race}
The race experiment was conducted on a long-flight of stairs. \figinitref{supp:race} visualizes the stair characteristics used in the experiment.
\begin{figure}[t!]
	\centering 
	\begin{subfigure}[b]{0.48\textwidth}
		\includegraphics[width=1.0\textwidth]{figures/supp/supp_race_red.pdf}
	\end{subfigure}
	% \captionsetup{font=footnotesize}
	\caption{\textbf{Geometrical details of the stairs used for robot race experiment.}}
	\label{figure:supp_race}
\end{figure}

To support the race experiments, we conducted additional asynchronous experiments where robot R4~(Fig.~\ref{figure:supp_hardware}C) was used to deploy the controllers. Robot~R4 was also controlled with an autonomous navigation module to ensure consistent path planning while climbing the stairs. The experiments videos are summarized in \mvone0, and a few snapshots of the experiments that highlight the robot's motions are shown in Fig.~\ref{figure:supp_async_race}. Robot~R4 was controlled using (\textbf{A})~DreamWaQ++, (\textbf{B})~DreamWaQ, and (\textbf{C})~Unitree Go1's built-in controller. The robot, controlled by DreamWaQ++, managed to climb the stairs with minimum leg and body collisions by adaptively raising its body and foot swing height. In contrast, the robot controlled with DreamWaQ experienced a series of stumbles, although it managed to climb the stairs due to the robust nature of the controller. The robot controlled by the Unitree Go1's built-in controller could climb the stairs but often got stuck due to the lack of adaptability in the controller.

One discernible behavior between DreamWaQ++ and DreamWaQ lies in its gait adaptation. DreamWaQ++ adapts its gait by raising its body and swinging its foot further to step on the stairs (see Fig.~\ref{figure:supp_async_race}A), while DreamWaQ tends to collide the robot foot with the stairs and then drag it along the stair's vertical surface before placing it on the next step (see Fig.~\ref{figure:supp_async_race}B). This behavior is less efficient and may cause the robot to stumble. On the other hand, the robot with Unitree Go1's built-in controller tends to use a fixed gait pattern, which is less adaptive to the stairs' geometry and lacks spatial memory, causing its rear leg to stumble multiple times (see Fig.~\ref{figure:supp_async_race}C).

\begin{figure}[t!]
	\centering 
	\begin{subfigure}[b]{0.48\textwidth}
		\includegraphics[width=1.0\textwidth]{figures/supp/supp_async_race_red.pdf}
	\end{subfigure}
	% \captionsetup{font=footnotesize}
	\caption{\textbf{Asynchronous stair-climbing experiments.} The robot was controlled using (\textbf{A}) DreamWaQ++, (\textbf{B}) DreamWaQ, and (\textbf{C})  Unitree Go1's built-in controller. The white mask on the stair indicates the same stair plate that each robot interacted with over the four successive snapshots. The full asynchronous race experiment is available in \mvone0.}
	\label{figure:supp_async_race}
\end{figure}

We also measured the state estimation error of the robot controlled by DreamWaQ++ and DreamWaQ during the asynchronous experiments. The state estimation error is the absolute error between the ground truth and estimated velocities. The ground truth data was obtained using a LiDAR odometry algorithm~\cite{xu2022fast}. The results are shown in Fig.~\ref{figure:supp_error_track}. The robot controlled by DreamWaQ++ exhibits a lower state estimation error compared to the robot controlled by DreamWaQ with a significant difference. This result indicates that the robot controlled by DreamWaQ++ can better estimate its position and adapt its gait to the stairs' geometry, which is crucial for climbing stairs efficiently, yielding a more stable and robust locomotion.

\begin{figure}[h!]
	\centering 
	\begin{subfigure}[b]{0.38\textwidth}
		\includegraphics[width=1.0\textwidth]{figures/supp/supp_vel_error_red.pdf}
	\end{subfigure}
	% \captionsetup{font=footnotesize}
	\caption{\textbf{Velocity estimation error comparison in the stair-climbing task.} The **** annotation indicates a significant difference between the two controllers as measured by a paired $t$-test.}
	\label{figure:supp_error_track}
\end{figure}

\subsection{Blind locomotion on stairs}\label{supp:dreamwaq}
We evaluate the performance of a blind locomotion controller trained using DreamWaQ~\cite{nahrendra2023dreamwaq} when traversing a series of stairs with $15\!\sim\!18~\mathrm{cm}$ high rise as shown in Fig.~\ref{figure:supp_dreamwaq}. Although the robot initially managed to climb the stairs, it became unstable due to a series of stumbles and eventually fell down before reaching the end of the stairs. We discovered that the most risky stumbles were when the two front legs stumbled at the same time, making the robot lose its balance. This result highlights the importance of exteroception for a legged robot to proficiently traverse through obstacles.

\begin{figure}[t!]
	\centering 
	\begin{subfigure}[b]{0.48\textwidth}
		\includegraphics[width=1.0\textwidth]{figures/supp/supp_stairs_red.pdf}
	\end{subfigure}
	% \captionsetup{font=footnotesize}
	\caption{\textbf{Illustrations of blind locomotion failure in a stair-climbing scenario.} A series of stumbles made the robot cannot preserve its stability and eventually fell down.}
	\label{figure:supp_dreamwaq}
\end{figure}

\subsection{Climbing a long flight of stairs}\label{supp:long_stairs}

\begin{figure}[t!]
	\centering 
	\begin{subfigure}[b]{0.48\textwidth}
		\includegraphics[width=1.0\textwidth]{figures/supp/supp_long_stairs_red.pdf}
	\end{subfigure}
	% \captionsetup{font=footnotesize}
	\caption{\textbf{Stairs climbing experiments}. The robot is commanded to climb a long flight of (\textbf{A})~straight and (\textbf{B})~curved stairs.}
	\label{figure:supp_long_stairs}
\end{figure}

\figinitref{figure:supp_long_stairs}E shows snapshots of the robot climbing $39$ steps of stairs, yielding a total elevation of $5.46~\textrm{m}$ and inclination of $25.76^{\circ}$. We used a blind locomotion controller trained using DreamWaQ as a baseline comparison. While the blind locomotion controller initially managed to overcome the stairs, its performance quickly deteriorated due to numerous stumbles (see supplementary section~\ref{supp:dreamwaq}). In contrast, the controller trained using DreamWaQ++ (Fig.~\ref{figure:supp_long_stairs}E) allowed the robot to swiftly climb the stairs with minimum leg and body collisions by adaptively raising its body and foot swing height. The robot reached the top of the stairs in $47~\textrm{s}$, stressing the importance of exteroception on locomotion over a long flight of stairs that necessitates fast adaptation of the robot's gait to minimize stumbles.

\subsection{Paired $t$-test on slope climbing}\label{supp:t-test}
The significance of the difference between torque exertion of each joint in Fig.~\ref{figure:results_adaptation}F was measured using a paired $t$-test method. The annotations on the figure are defined based on the resulting $p$-values. We follow the standard rule defined in Table~\ref{table:t-test}. The $p$-values were corrected using the Bonferroni correction method~\cite{florian_charlier_2022_7213391} and presented in Table~\ref{table:p-value}.

% ===================================================================================
\begin{table}[t!]
% \begin{threeparttable}
\caption{Description for $p$-value annotation~\cite{florian_charlier_2022_7213391}.}
\centering
% \captionsetup{justification=centering}

\label{table:t-test}
\begin{center}
\begin{tabular}{lll}
\hline \hline
Annotation           & Criteria \\ \hline 
ns (not significant)  &                      $0.05 < p \leq 1.0$ \\
$*$  &                      $0.01 < p \leq 0.05$ \\
$**$  &                      $0.001 < p \leq 0.0$ \\
$***$  &                      $0.0001 < p \leq 0.001$ \\
$****$  &                      $ p \leq 0.0001$ \\
\hline \hline
\end{tabular}
\end{center}
\end{table}
% ===================================================================================

% ===================================================================================
\begin{table}[t!]
% \begin{threeparttable}
\centering
% \captionsetup{justification=centering}
\caption{$p$-value results of data reported in Fig.~\ref{figure:results_adaptation}.}
\label{table:p-value}

\begin{center}
\begin{tabular}{llc}
\hline \hline
Joint           & $p$-value & Signficance \\ \hline 
FR Thigh  &                      $1.0$ 			& ns\\  
FR Calf  &                      $0.4464$ & ns\\  
FL Thigh  &                      $1.0$ & ns\\  
FL Calf  &                      $1.0$ & ns\\  
RR Thigh  &                      $0.001244$ & **\\  
RR Calf  &                      $0.00009325$ & ****\\  
RL Thigh  &                      $0.00001922$ & ****\\  
RL Calf  &                      $1.0$ & ns\\  
\hline \hline
\end{tabular}
\end{center}
\end{table}
% ===================================================================================

\subsection{Exteroception preprocessing}\label{supp:exteroception_preprocessing}
In this work, we employ a voxel grid representation as the input for the policy. The voxel grid encompasses downsampled robot-centric 3D points obtained from an exteroceptive sensor mounted on the robot. The voxels are obtained via voxel-grid filtering with a leaf size of $0.05~\mathrm{m}$. We assume accurate extrinsic calibration parameters are available to transform the measured 3D points from the sensor frame to the body frame. We set the exteroceptive measurements to be within a grid with its row and column size of $w\!=\!1.1~\mathrm{m}$ and $h\!=\!0.5~\mathrm{m}$, respectively. The first row of the grid is located $0.9~\mathrm{m}$ in front of the robot, yielding a grid with 10 rows and 22 columns by dividing the size with the leaf size.

\subsection{Constrained reparameterization trick}\label{supp:constrained_reparam}
The multi-modal encoder architecture encompasses multiple stochastic layers within the encoders and multi-modal mixer networks, offering advantages such as enhanced robustness and increased exploration capabilities. However, a trade-off arises with numerical stability during the early stages of training. 

A straightforward solution is to balance the weight of the reconstruction loss and KL divergence in $\mathcal{L}_\mathrm{VAE}$. In variational inference, the prior distribution of the latent state is often assumed to follow a normal distribution. The stability issue can be mitigated by putting more emphasis on the latent loss during training. This approach ensures that the encoder learns a better approximation of the latent space while preserving the ability to reconstruct the input data accurately.

However, strongly matching the posterior and prior distributions via the latent loss can lead to another issue where the encoder tends to neglect important details in the input point cloud. This deficiency makes the policy unable to detect and respond to small obstacles in the environment effectively. To overcome this challenge, we introduced a constrained reparameterization trick, defined as

\begin{equation}
    \textbf{z} \sim N(g_{\mu}(\textbf{x}),g_{\sigma}(\textbf{x})),
\end{equation}
where $\textbf{z}$ is a stochastic latent vector and $\textbf{x}$ is the input of the encoder network $g$. The subscripts $\mu$ and $\sigma$ indicate the outputs of $g(x)$ that correspond to the mean and standard deviation of the latent distribution, respectively. $z$ is sampled from a Gaussian distribution $N(\cdot,\cdot)$ with mean $g_{\mu}(\textbf{x})$ and standard deviation $g_{\sigma}(\textbf{x})$. 

During this reparameterization step, we imposed hard constraints on the standard deviation of the distribution, such that $\sigma_\mathrm{min}\leq g_{\sigma}(\textbf{x}) \leq \sigma_\mathrm{max}$. This constraint ensures that the generated samples are numerically stable and can be reliably propagated to the subsequent layers of the network. By implementing this simple yet effective solution, the learning process becomes much more stable without compromising the final performance of the learned policy. Empirically, we set $\sigma_\mathrm{min}=0$ and $\sigma_\mathrm{max}=5$ to promote stable training. This constrained reparameterization trick is employed on all encoder networks that utilize a stochastic layer.

\subsection{Training environment details} \label{supp:training_env}
\subsubsection{\textit{Simulation}}
We used NVIDIA Isaac Gym~\cite{makoviychuk2021isaac} preview 3 as the simulator for training the controller and multi-modal context encoder networks. The training environments were built upon the Legged Gym library~\cite{rudin2021learning}. We employed domain randomization over $3,\!500$ agents, which took about 11 hours of training on an NVIDIA A5000 GPU. Afterwards, the trained networks were deployed without any fine-tuning on a real or simulated robot in the Gazebo simulation for the evaluations presented in this paper. 

\subsubsection{\textit{Control pipeline}}
The policy and multi-modal context encoder networks ran synchronously while receiving asynchronous observations. Proprioceptive measurements were sampled at $200~\textrm{Hz}$, whereas exteroceptive measurements were sampled at $10~\textrm{Hz}$. The controller integrated the most recent measurements, operating at $50~\textrm{Hz}$. To enhance the robustness of the controller against the asynchronous observations, we employed latency randomization during training. Detailed information regarding the randomized latency for all measurements is provided in Table~\ref{table:domain_randomization}.

The policy network generated target joint positions at a rate of $50~\textrm{Hz}$, which were subsequently transmitted to a low-level proportional-derivative (PD) controller operating at $200~\textrm{Hz}$. Within the PD controller, the target joint positions were converted into torque commands, employing proportional ($K_p$) and derivative ($K_d$) control gains of $25$ and $0.7$, respectively. These computed torque commands were subsequently relayed to the low-level motor controller integrated within our customized Unitree Legged SDK.

% \begin{itemize}
%     \item \textbf{Rough slopes} are generated by
%     \item \textbf{Stairs}
%     \item \textbf{Gaps}
%     \item \textbf{Random discrete}
% \end{itemize}

\subsubsection{\textit{Curriculum}}
We leveraged three curriculums during training, i.e.~terrain, command, and reward curriculums. For the terrain curriculum, several terrains were procedurally generated at the beginning of training to simulate various obstacles the robot might encounter in the real world. The terrain curriculum utilized the game-inspired curriculum setting~\cite{rudin2021learning} with ten different levels of difficulty. We generally utilized \texttt{rough}, \texttt{stairs}, \texttt{gaps}, and \texttt{discretized obstacle} terrains to introduce variations in the exteroception, which could induce diversity in the training data for the multi-modal context encoder. An agent was promoted to the next level if it could traverse more than half of the distance at the current level. When an agent failed to traverse more than half of the distance at the current level for more than ten episodes, it was demoted to the previous level. If an agent successfully walked through all levels, it will be randomly spawned within the ten levels, preventing catastrophic forgetting and diversifying the training data.
 
The policy was trained to maximize the command tracking rewards while satisfying style rewards (Table~\ref{table:reward_functions}), resulting in smooth and accurate robot motion. The curriculum was a reward-based one, which automatically increased the command velocity range when the velocity tracking reward, $r_{v_{x,y}}\in[0, 1]$, surpassed a given threshold, $r^\textrm{thres}_{v_{x,y}}$, which was set to $0.9$. 

Finally, the reward curriculum ensures safe behavior in the real world by gradually increasing the penalty for the style rewards. Applying strong penalties to the style rewards at early training can restrict exploration, resulting in poor performance. However, without a strong penalty, the robot tends to behave aggressively once noisy exteroceptive measurements are taken as inputs in the real world. Hence, a reward curriculum that exponentially grows over learning iteration was utilized to facilitate stable learning. More details are provided in section~\ref{supp:reward_functions}.

\subsubsection{\textit{Domain randomization}}
We randomized multiple physical properties of the robot and the environment to facilitate sim--to--real transfer. Additionally, we employed Roll-Drop~\cite{campanaro2023roll} to encourage exploration and robustness on top of physics randomization. Details of the physical properties and its randomization ranges are provided in Table~\ref{table:domain_randomization}.

\begin{table}[t!]
\centering
% \captionsetup{justification=centering}
\caption{Domain randomization ranges applied in the simulation.}
\label{table:domain_randomization}
\begin{center}
\begin{tabular}{lccc}
\hline\hline
Parameter                        & Randomization range & Unit \\\hline
Payload                     & $[-1, 2]$ & $\mathrm{~kg}$     \\ 
$K_p$ factor   & $[0.9, 1.1]$ & $\mathrm{~Nm~rad^{-1}}$    \\ 
$K_d$ factor        & $[0.9, 1.1]$ & $\mathrm{~Nms~rad^{-1}}$   \\ 
Motor strength factor        & $[0.9, 1.1]$ & $\mathrm{~Nm}$   \\ 
Center of mass shift        & $[-50,50]$ & $\mathrm{~mm}$    \\
Friction coefficient        & $[0.2, 1.25]$ & -    \\
System delay                        & $[0.0, 15.0]$ &  $\mathrm{~ms}$   \\

\hline\hline
\end{tabular}
\end{center}
\vspace{-0.cm}
\end{table}

\subsubsection{\textit{Adversarial observation}}
We injected noises into the proprioceptive and exteroceptive observations. For the proprioceptive observations, a uniform noise was injected at each time step. 
% The magnitude of noises for each observation \rvc{is} summarized in Table~\ref{table:observation_noise}. 
For the exteroceptive data, we classified three different noise ranges, constituting low, medium, and high noises. The proportion of these exteroceptive noise scales was set to $30\%$, $50\%$, and $20\%$, respectively.
The magnitude of noises for each observation is summarized in Table~\ref{table:observation_noise}. 

\begin{table}[t!]
\centering
% \captionsetup{justification=centering}
\caption{Noise parameters injected into the observation for the policy network during training.}
\label{table:observation_noise}
\begin{center}
\begin{tabular}{lccc}
\hline\hline
Observation                        & Noise range ($\mu$) & Unit \\\hline
Joint position  &                      $[-0.01, 0.01]$ & $\mathrm{rad}$     \\ 
Joint velocity  &                      $[-1.5, 1.5]$ & $\mathrm{rad/s}$    \\ % $\mathrm{rad~s^{-1}}$    \\ 
Body linear velocity &                 $[-0.1, 0.1]$ & $\mathrm{m/s}$   \\ % $\mathrm{m~s^{-1}}$   \\ 
Body angular velocity &                $[-0.2, 0.2]$ & $\mathrm{rad~^{-1}}$   \\ 
Gravity vector        &                $[-0.05, 0.5]$ & $\mathrm{m/s^{2}}$    \\ % $\mathrm{m~s^{-2}}$    \\
Exteroceptive measurement (low)  &     $[0.0, 0.03]$ & $\mathrm{m}$\\
Exteroceptive measurement (medium)  &     $[0.03, 0.1]$ & $\mathrm{m}$    \\
Exteroceptive measurement (high)  &     $[0.1, 0.3]$ & $\mathrm{m}$    \\

\hline\hline
\end{tabular}
\end{center}
\vspace{-0.cm}
\end{table}

Although observation noise is often easily handled by a controller that leverages only proprioception if trained with sufficient domain randomization,  the learned controller exhibited increased sensitivity to disturbances in exteroception, primarily attributed to the rich information contained within exteroceptive measurements. Several issues, such as inaccurate extrinsic calibration and sensor noise, significantly deteriorated the controller's robustness. In robotics, auto-calibration is a highly desirable attribute, capable of enhancing system robustness. Consequently, we aimed to integrate this capability into the proposed multi-modal context encoder.

To achieve this, we trained the multi-modal context encoder to explicitly predict extrinsic calibration errors within the exteroception data. This explicit error prediction serves a dual purpose within our framework. First, it provides guidance to human operators, enabling them to recalibrate the extrinsic parameters effectively. Concurrently, the multi-modal context encoder learns to discern and mitigate the impact of this calibration error, thus producing more accurate exteroception reconstructions. This proactive approach enhances the overall performance and resilience of the proposed system in the presence of exteroceptive disturbances.

Throughout the training process, we introduced a randomization procedure for the extrinsic calibration parameters within the $SE(3)$ coordinate system at the beginning of each episode. These calibration parameters served as ground-truth values, challenging the multi-modal context encoder to predict them accurately. We proposed a customized perturbation model for the exteroception because we are exploiting the robot-centric height scan as the input for the encoder. The perturbation model consists of i) noise, ii) sensor alignment error, and iii) pruning.

\paragraph{Noise model}
The noise model is designed to mimic the characteristics of range measurement sensors such as LiDAR \rvc{sensors} or depth cameras. First, the distance between the sampled 3D robot-centric points to the body frame of the robot is measured as $\textbf{d}_t=[d^1_t\;\cdots{}\;d^i_t\;\cdots{}\;d^I_t] \in \mathbb{R}^{1 \times I}$, where $i$ indicates the $i$-th element and $I$~is the number of points per scan. 
Then, for the $i$-th point, an anisotropic Gaussian noise is applied to the point set $\textbf{p}_t=[\textbf{p}^1_t\;\cdots\;\textbf{p}^i_t\;\cdots\;\textbf{p}^I_t]\in\mathbb{R}^{3 \times I}$, where $\textbf{p}^i_t=\begin{bmatrix} x^i_t & y^i_t &  z^i_t \end{bmatrix}$. The Gaussian noise is centered at the nominal noise level, and the variance is scaled according to the distance of each point to the robot. Practically, exteroceptive measurements in the real world exhibit higher noise when the terrains are very close to the sensor. Therefore, we formulate each noisy point as

\begin{equation}
    \textbf{p}^i_t = 
    \begin{bmatrix}
    x^i_t + \mathcal{N}\left(\mu_x, \sigma^2_x\right)\\
    y^i_t + \mathcal{N}\left(\mu_y, \sigma^2_y\right)\\
    z^i_t + \mathcal{N}\left(\mu_z, \sigma^2_z\right)\\
    \end{bmatrix},
    \label{eq:noise_model}
\end{equation}
where $\mu$  and $\sigma^2$ are the nominal noise level and noise variance, respectively, with the subscripts $x$, $y$, and $z$ indicating that the elements correspond to the $x$, $y$, and $z$ axes. These noise parameters were sampled from a uniform distribution within the range specified in Table~\ref{table:point_noise} at the beginning of every episode. Afterwards, the point-wise noise in~\eqref{eq:noise_model} was sampled at every time step.

\begin{table}[t!]
\centering
% \captionsetup{justification=centering}
\caption{Point noise parameters during training.}
\label{table:point_noise}
\begin{center}
\begin{tabular}{cccc}
\hline\hline
Parameter                        & Range & Unit \\\hline
$\mu_x$  &                      $[0.0, 2.0]$ & $\mathrm{cm}$     \\ 
$\mu_y$  &                      $[0.0, 2.0]$ & $\mathrm{cm}$    \\ % $\mathrm{rad~s^{-1}}$    \\ 
$\mu_z$ &                       $[0.0, 5.0]$ & $\mathrm{cm}$   \\ % $\mathrm{m~s^{-1}}$   \\ 
$\sigma_x$ &                    $[0.0, 1.0]$ & $\mathrm{cm}$   \\ 
$\sigma_y$        &             $[0.0, 1.0]$ & $\mathrm{cm}$    \\ % $\mathrm{m~s^{-2}}$    \\
$\sigma_z$  &                   $[0.0, 3.0]$ & $\mathrm{cm}$\\

\hline\hline
\end{tabular}
\end{center}
\vspace{-0.cm}
\end{table}

\paragraph{Sensor alignment bias}
We applied sensor alignment bias at the beginning of each episode to simulate extrinsic calibration error. This error included positional and rotational errors, i.e. $\begin{bmatrix} \Delta x, & \Delta y, & \Delta z, & \Delta \mathrm{roll}, & \Delta \mathrm{pitch}, & \Delta \mathrm{yaw} \end{bmatrix}$. The alignment errors were sampled from a uniform distribution and consistently applied to the measured points throughout the episode. The alignment bias parameters are summarized in Table~\ref{table:alignment_bias}.

% ===================================================================================
\begin{table}[t!]
% \begin{threeparttable}
\centering
\captionsetup{singlelinecheck=false}
\caption{Sensor alignment bias between the body frame of exteroceptive sensor and robot.}
\label{table:alignment_bias}

\begin{center}
\begin{tabular}{ccc}
\hline \hline
\multicolumn{1}{c}{Parameter} & Error range & Unit  \\\hline 
$\mathrm{roll}$             & $[-0.2, 0.2]$ &  $\mathrm{rad}$   \\
$\mathrm{pitch}$            & $[-0.15, 0.15]$ &  $\mathrm{rad}$   \\
$\mathrm{yaw}$              & $[-0.1, 0.1]$ &  $\mathrm{rad}$   \\
$\mathrm{x}$             & $[-0.1, 0.1]$ &  $\mathrm{m}$   \\
$\mathrm{y}$             & $[-0.1, 0.1]$ &  $\mathrm{m}$   \\
$\mathrm{z}$             & $[-0.1, 0.1]$ &  $\mathrm{m}$   \\
\hline \hline      
\end{tabular}
\end{center}
\end{table}
% ===================================================================================

\paragraph{Pruning}
The major distinction between the height scans sampled in simulation and those obtained from real-world exteroceptive sensors is the presence of inherent blind spots in the latter. These blind spots can result from either the sensor's specifications or its placement on the robot, leading to occlusion by certain robot parts. One of the possible solutions to this problem is by employing raycasting from the sensor pose to the sampled height scan. However, this solution can be computationally expensive and greatly affect simulation time. In this work, we employed a simpler solution to eliminate or \textit{prune} parts of the exteroceptive data before it was fed into the multi-modal context encoder.

First, we construct a probability masking layer to prune the exteroceptive measurement that has been preprocessed using the method detailed in section~\ref{supp:exteroception_preprocessing}. During locomotion on the flat terrain, appropriately positioned exteroceptive sensors should effectively measure the terrain within a pre-defined grid area. However, the reliability of these measurements diminishes when the robot encounters obstacles or pits. To address this challenge, we introduced a probability masking technique that assigns a higher pruning probability to points that are distant and elevated or close and low to the robot. This pruning strategy makes a setting that allows the multi-modal context encoder to learn point completion from sparse exteroceptive inputs.

\subsubsection{\textit{Privileged states}}
For the privileged exteroception, we use a robot-centric local height map sampled around the robot. The local map is a 2.5D grid, where each value of the grid represents the height of the terrain on the corresponding grid. The grid is constructed with its row and column size of $w\!=\!1.1~\mathrm{m}$ and $h\!=\!1.7~\mathrm{m}$, respectively. The first row of the grid is located $0.9~\mathrm{m}$ in front of the robot's body frame, similar to the 3D voxel grid for the multi-modal encoder's input. The resolution of the grid is set to $5~\mathrm{cm}$.

For the privileged proprioception, we provide ground truth and noiseless measurements as follows:
\begin{enumerate}
    \item Gravity vector on the robot's body frame.
    \item Body linear and angular velocities.
    \item Joint positions and angular velocities.
    \item External disturbance force and torque applied to the robot's body frame.
    \item Physical properties (friction, motor damping, motor stiffness, motor strength ratio, additional payload, and the robot's center of mass).
    \item Foot position relative to the robot's body frame.
\end{enumerate}

\subsection{Reward functions}\label{supp:reward_functions}
Table~\ref{table:reward_functions} lists all the reward functions,~$\textbf{r}$, used in DreamWaQ++, which are mainly based on the rewards used in~\cite{nahrendra2023dreamwaq}. On top of these rewards, we also employed a reward curriculum to exponentially anneal some style rewards, i.e.~joint torque, joint velocity, joint acceleration, action rate, and smoothness rewards. The annealing rule follows the following formula:

\begin{equation}
    w_{i+1}=\lambda w_{i},
\end{equation}
where $w$ is the reward weight, $i$ is the learning iteration, and $\lambda$ is the annealing rate. We set $\lambda\!=0.998$
and $w_0$ for the selected skill rewards are summarized in Table~\ref{table:reward_init}.
% ===================================================================================
\begin{table}[t!]
% \begin{threeparttable} 
\centering
\captionsetup{singlelinecheck=false}
\caption{Reward function elements and their corresponding weights. $\mathrm{exp(\cdot)}$ and $\mathrm{var(\cdot)}$ are exponential and variance operators, respectively. $(\cdot)^\mathrm{des}$ and $(\cdot)^\mathrm{cmd}$ indicate the desired and commanded values, respectively. $x, y,$ and $z$ are defined on the robot's body frame, with $x$ and $z$ pointing forward and upward, respectively. $\textbf{g}$, $\textbf{v}_{xy}$, $\omega_\mathrm{yaw}$, $h$, $p_{f,z,k}$, $v_{f,xy,k}$, and $\boldsymbol{\tau}$ are the gravity vector projected into the robot's body frame, linear velocity vector in the $xy$ plane, yaw rate, body height w.r.t. the ground, foot height, foot lateral velocity, and joint torque, respectively.}
\label{table:reward_functions}

\begin{center}
\begin{tabular}{lll}
\hline \hline
Reward           & Equation ($\textbf{r}$) & Weight ($w$) \\ \hline 
\multicolumn{3}{l} {\textit{Task rewards}}           \\ 
Lin. velocity tracking  & $\exp{\{-4(\textbf{v}^\mathrm{cmd}_{xy}-\textbf{v}_{xy})^{2}\}}$ & $1.0$      \\ 
Ang. velocity tracking & $\exp{\{-4(\omega^\mathrm{cmd}_\mathrm{yaw}-\omega_\mathrm{yaw})^{2}\}}$ & $0.5$ \\ \hline
\multicolumn{3}{l} {\textit{Style rewards}}           \\ 
Linear velocity ($z$) & $v^2_z$ & $-2.0$ \\
Angular velocity ($xy$) & $\boldsymbol{\omega}^2_{xy}$ & $-0.05$ \\
Uprightness & $|\textbf{g}|^2$ & $-0.2$ \\
Joint acceleration & $\boldsymbol{\ddot{\theta}}^2$ & $-2.5\!\times\!10^{-7}$ \\
Joint power & $|\boldsymbol{\tau}||\boldsymbol{\dot{\theta}}|$ & $-2\!\times\!10^{-5}$ \\
Body height & $(h^\text{des}-h)^2$ & $-1.0$ \\
Foot clearance & $(p^\text{des}_{f,z,k}-p_{f,z,k})^2\cdot v_{f,xy,k}$& $-0.01$ \\
Action rate & $(\textbf{a}_t - \textbf{a}_{t-1})^2$ & $-0.01$ \\
Smoothness & $(\textbf{a}_t - 2\textbf{a}_{t-1} + \textbf{a}_{t-2})^2$& $-0.01$ \\
Power distribution &$\mathrm{var}(\boldsymbol{\tau}\cdot\boldsymbol{\dot{\theta}})^2$ & $-10^{-5}$ \\ 
\hline \hline
\end{tabular}
\end{center}
\end{table}
% ===================================================================================

% ===================================================================================
\begin{table}[t!]
% \begin{threeparttable}
\centering
\captionsetup{singlelinecheck=false}
\caption{Initial weight $w_0$ for selected style rewards that were annealed using the reward curriculum.}
\label{table:reward_init}

\begin{center}
\begin{tabular}{lll}
\hline \hline
Reward           & Weight ($w_0$)\\ \hline 
Joint torque & $-5\!\times\!10^{-6}$ \\
Joint velocity & $-6\!\times\!10^{-6}$ \\
Joint acceleration & $-7.5\!\times\!10^{-8}$ \\
Action rate & $-1.5\!\times\!10^{-5}$ \\
Smoothness & $-1.5\!\times\!10^{-5}$ \\
\hline \hline
\end{tabular}
\end{center}
\end{table}
% ===================================================================================

\subsection{Embedding analysis}\label{supp:embedding_analysis}
\subsubsection{Evaluation setting}
We conducted an embedding analysis on the context vector generated by the encoder. This analysis was carried out using data acquired within a simulation-to-simulation (sim-to-sim) setup. In this setup, both the fully trained encoder and policy networks were deployed within a Gazebo simulator. We implemented four distinct terrain types to facilitate this evaluation, as depicted in Fig.~\ref{figure:supp_gazebo_terrain}. In this setting, the stair difficulties are parameterized by its \textit{rise} and \textit{run}, i.e.~its vertical and horizontal dimensions, respectively~\cite{barasuolstair}. Easy stairs have low rise and high run values, while hard stairs have high rise and low run values.

\begin{figure}[t!]
	\centering 
	\begin{subfigure}[b]{0.48\textwidth}
		\includegraphics[width=1.0\textwidth]{figures/supp/gazebo_terrain_red.pdf}
	\end{subfigure}
	% \captionsetup{font=footnotesize}
	\caption{\textbf{Illustrations of terrains used for evaluation in the Gazebo simulator.} Four types of terrains were constructed to evaluate the change in values of the context features. 
    % Four types of terrains were constructed to evaluate the changes in values of the context features. 
    The world model employed for this evaluation is an adapted version of the simulation model utilized in the IEEE ICRA 2023 Autonomous Quadrupedal Robot Challenge~\cite{jacoff2023taking}.}
	\label{figure:supp_gazebo_terrain}
\end{figure}

\subsubsection{Visualization via dimension reduction}
We performed dimensionality reduction on the proprioceptive, exteroceptive, and multi-modal contexts to depict their distributions within a 2D space. While one of the prevailing approaches for embedding visualization involves t-distributed stochastic neighbor embedding (t-SNE)~\cite{van2008visualizing}, it is worth noting that t-SNE, despite yielding satisfactory cluster visualizations, is notably less efficient at capturing overarching embedding structures. Its emphasis lies predominantly on local structures, potentially leading to inadequate comprehension of meaningful information within multi-modal data. Consequently, this limitation of t-SNE may hinder the comprehensive insights required for thorough analysis.

Hence, we extended our approach to dimensionality reduction by employing PaCMAP~\cite{wang2021understanding}, a recently introduced technique that offers a more balanced preservation of both local and global embedding structures. In this manner, we achieved visualizations of the embeddings within a 2D space for diverse terrains (as exemplified in Fig.~\ref{figure:supp_gazebo_terrain}). The visualization results are presented in Fig.~\ref{figure:supp_embedding_noblind}.

\begin{figure}[t!]
	\centering 
	\begin{subfigure}[b]{0.48\textwidth}
		\includegraphics[width=1.0\textwidth]{figures/supp/supp_noblind_embedding_red.pdf}
	\end{subfigure}
	% \captionsetup{font=footnotesize}
	\caption{\textbf{2D visualization of the embeddings after dimensionality reduction.}}
	\label{figure:supp_embedding_noblind}
\end{figure}

As anticipated, the t-SNE method effectively portrays the exteroceptive context, revealing discernible clusters that imply the disentangled latent representation of different terrains. However, interpreting the proprioceptive context poses challenges in providing a coherent understanding. Consequently, the visualization of the multi-modal context fails to yield significant insights, aside from distant clusters indicative of varying terrains encoded in the exteroceptive context.

Meanwhile, PaCMAP more explicitly captures fundamental intrinsic characteristics of the embedding~\cite{wang2021understanding}. Within the proprioceptive context, PaCMAP effectively illustrates circular clusters, which plausibly correspond to the cyclic gait patterns exhibited by the robot's feet. An interesting observation arises as the circular radius expands on less challenging terrains. Our conjecture aligns with the notion that this radius could indicate the gait's duty cycle or swing time, as on smoother terrains without obstacles, the robot's feet undergo extended swing durations.

Our embedding analysis showcases that the structured representation learning facilitated by our context encoder yields informative latent variables without necessitating explicit estimation of physical attributes. As postulated by Nahrendra \textit{et al.}~\cite{nahrendra2023dreamwaq}, the unsupervised representation learning mechanism empowers the encoder to encode informative latent features while maintaining dynamic feature interactions selectively. The mechanism inherent in our context encoder thus amalgamates the best of both approaches, eliminating the requirement for manual and explicit selection of estimated variables while concurrently generating structured and disentangled latent representations.

\begin{figure}[t!]
	\centering 
	\begin{subfigure}[b]{0.48\textwidth}
		\includegraphics[width=1.0\textwidth]{figures/supp/supp_blind_embedding_red.pdf}
	\end{subfigure}
	% \captionsetup{font=footnotesize}
	\caption{\textbf{2D visualization of the dimension-reduced embeddings during blind locomotion.}}
	\label{figure:supp_embedding_blind}
\end{figure}

We extended our embedding analysis to the blind locomotion scenario using our framework. In this assessment, we collected data by disabling exteroception, providing constant flat terrain points, and commanding the robot to walk across various terrains, as depicted in Fig.~\ref{figure:supp_embedding_blind}. The t-SNE visualization outcomes, while potentially sufficient for the policy network, remain less straightforward for practical interpretation. Such results could mislead practitioners into erroneously concluding that the encoder has not effectively learned a disentangled context vector.

In contrast, the PaCMAP visualization method successfully captures meaningful structures within the proprioceptive context. During blind locomotion, the proprioceptive context plays an important role because it remains the sole modality that the policy can rely on. As illustrated in Fig.~\ref{figure:supp_embedding_blind}, the proprioceptive context captures local structures induced by the robot's feet motions similar to the non-blind scenario. This distinctiveness becomes more discernible upon mixing into a multi-modal context, even when fused with the false exteroceptive context obtained in the blind locomotion scenario.

\subsubsection{Effect of contrastive loss}
\begin{figure}[t!]
	\centering 
	\begin{subfigure}[b]{0.48\textwidth}
		\includegraphics[width=1.0\textwidth]{figures/supp/supp_contrastive_red.pdf}
	\end{subfigure}
	% \captionsetup{font=footnotesize}
	\caption{\textbf{Effect of contrastive loss in the learned embedding.} The embeddings are recorded from locomotion on flat, irregular, easy stairs, and hard stairs terrains. The comparison shows the nature of the embedding when the contrastive loss is removed or retained.}
	\label{figure:supp_contrastive}
\end{figure}

We further investigated the impact of the contrastive loss on the learned embedding. The contrastive loss is a crucial component in training the multi-modal context encoder because it encourages the encoder to learn a structured representation. To evaluate the effect of the contrastive loss, we trained the encoder without the contrastive loss and compared the learned embeddings with those obtained from the full training setup using the contrastive loss. The results are depicted in Fig.~\ref{figure:supp_contrastive}.

The comparison showed that the contrastive loss significantly influences the learned embedding. The embeddings obtained from the full training setup exhibit more structured and disentangled latent variables than those obtained without contrastive loss. Indeed, some structured patterns in the embeddings are still discernible without the contrastive loss, mostly attributed to the exteroceptive data that provides spatial information. However, it fails to capture lower-level circular patterns in the proprioceptive data, which is crucial for the robot's locomotion. This observation underscores the importance of contrastive loss in the training of the multi-modal context encoder, as it facilitates the learning of structured and disentangled latent variables essential for the robot's locomotion.

\subsubsection{Attribution of latent variables}
\begin{figure}[t!]
	\centering 
	\begin{subfigure}[b]{0.48\textwidth}
		\includegraphics[width=1.0\textwidth]{figures/supp/supp_attribution_red.pdf}
	\end{subfigure}
	% \captionsetup{font=footnotesize}
	\caption{\textbf{Boxplot of each embedding variable in the multi-modal context vector.} The embeddings are recorded from locomotion on \textbf{(A)} flat, \textbf{(B)} irregular, \textbf{(C)} easy stairs, and \textbf{(D)} hard stairs terrains.}
	\label{figure:supp_embedding_attribution}
\end{figure}
We utilized boxplots to portray the raw embedding values, facilitating the analysis of their distribution as the robot navigates diverse terrains. The boxplot depicted in Fig.~\ref{figure:supp_embedding_attribution} reveals intriguing trends within the exteroceptive context. Particularly noteworthy are four embedding variables ($41$, $42$, $55$, and $64$th embeddings) exhibiting significantly expansive distributions. We posit that these characteristics are closely tied to the robot's foot motion while traversing terrains of varying complexities. To substantiate this hypothesis, we conducted an experiment involving scaling these four embedding variables before being fed to the policy network. This scaling operation involved adjustments of $0.1$ and $3.0$ times their original values to investigate the effect that it may bring to the robot's foot motions.

\begin{figure}[t!]
	\centering 
	\begin{subfigure}[b]{0.48\textwidth}
		\includegraphics[width=1.0\textwidth]{figures/supp/latent_modulation_red.pdf}
	\end{subfigure}
	% \captionsetup{font=footnotesize}
	\caption{\textbf{Latent modulation on some of the exteroceptive embedding proportionally affects the gait height.} The robot exhibits different locomotion styles when particular latent variables ($41$, $42$, $55$, and $64$th embeddings) were scaled with (\textbf{A}) $0.1$, (\textbf{B}) $1.0$, and (\textbf{C}) $3.0$ times of its original value. The difference resulted from this modulation is observable from the FR foot's $z$ position w.r.t. the base as shown in Fig.~\ref{figure:results_terrain}C.}
	\label{figure:supp_latent_modulation}
\end{figure}

This discovery shown in Fig.~\ref{figure:supp_latent_modulation} emphatically underscores the efficacy of structured representation learning, wherein essential physical attributes are embodied via an unsupervised approach. Moreover, this behavior offers a novel insight into the realm of interpretable learning-based control, countering the conventional notion of modern deep reinforcement learning as a ``black box'' system devoid of user-accessible modulations. Our findings demonstrate that structured representation learning engenders the acquisition of structured embeddings that can be flexibly modulated, enabling the generation of diverse behaviors by manipulating the intermediate embedding variables. This property opens up compelling possibilities for bridging the gap between learned locomotion controllers and their model-based counterparts. It also enables intuitive tuning by a human operator or a higher-level planner. 

Importantly, this property naturally emerged and was not explicitly specified during training or in the input command for the controller, distinguishing our work from that of Margolis~\textit{et al}.~\cite{margolis2022walk} that explicitly gives a style command into the policy network. Instead, this interpretable latent structure arose from the structured representation learning facilitated by the multi-modal context encoder within the proposed framework. 

However, we note that while the observed trend remains consistent, the indices of the modulated latent and its scale consistently change with different training seeds. This variability is expected because we do not enforce the learning of these variables in a supervised manner. 

% Instead, these variables are acquired through an unsupervised yet structured learning framework of the multi-modal context encoder, which enables the discovery of interpretable latent variables.

\subsubsection{Embedding feature-wise cross-correlation}
The heatmap plots shown in Fig.~\ref{figure:results_terrain}D underscore the efficiency of the multi-modal context encoder, which dynamically encodes multi-modal perception without any bias toward a particular modality. The multi-modal context encoder adaptively shifts its attention to modalities that provide the most informative priors for the policy. Furthermore, the notion of cross-modal correlation introduces interpretability on the uncertainties faced by the context encoder. This uncertainty measurement is particularly beneficial for higher-level modules. For instance, the uncertainty measurement can be leveraged by a traversability mapping module to adaptively shift its reliance on different sensor modalities for map update.

\subsection{Sensor--agnostic deployment}\label{supp:sensor_agnostic}
A fundamental strength of the policy trained using DreamWaQ++ is its sensor-agnostic property. The policy and context encoder were jointly trained in the simulation without any specific sensor model but only leveraged 3D points scan in front of the robot. Hence, the learned networks can be deployed on the real robot without any further training procedure. The only calibration required is the extrinsic parameters that transform 3D points from the sensor to the robot's body frame. This approach makes our method more simple and efficient than other existing works that rely on distilling a teacher policy into a student policy to bridge the gap between simulation and real-world exteroception. Furthermore, given that the context encoder was trained using 3D points as its input, it does not require any assumption on the number of points or grids. Instead, it will learn to infer the reliability of the exteroception and construct an informative latent feature for the policy. 

We performed an experiment using robot R3 to verify the adaptability of the learned controller to different sensor configurations. In this experiment, we built a local map surrounding the robot because we had access to stronger computation power, as well as an onboard LiDAR sensor on robot~R3. We constructed a local map of size $1.7\;\mathrm{m}\times1.1\;\mathrm{m}$ with a $0.1\;\mathrm{m}$ resolution. 

\begin{figure}[t!]
	\centering 
	\begin{subfigure}[b]{0.48\textwidth}
		\includegraphics[width=1.0\textwidth]{figures/supp/supp_sensor_agnostic_red.pdf}
	\end{subfigure}
	% \captionsetup{font=footnotesize}
	\caption{\textbf{Sensor agnostic deployment.} (\textbf{A}) Adaptability of the perception networks in different exteroceptive data settings. Despite the controller being trained solely with front-facing points, as depicted in Fig.~\ref{figure:dreamwaqpp}, it demonstrates adaptability to 3D point inputs that encompass the robot (illustrated with red points). The reconstruction of these points (represented by blue points) accurately captures the geometric properties of the robot's surroundings.} (\textbf{B})~A real-world stair-climbing experiment, which validates the adaptability of the controller when different exteroceptive configurations are used for the controller.
	\label{figure:supp_sensor_agnostic}
\end{figure}

\figinitref{figure:supp_sensor_agnostic}A shows the local map input (red dots) and its reconstruction (blue dots). Despite never trained with such exteroceptive setting, the encoder and decoder networks can still reconstruct the map with a satisfactory accuracy. The adaptability of the controller was further verified through a stair-climbing experiment in Fig.~\ref{figure:supp_sensor_agnostic}B. The robot can resiliently climb the stairs and by utilizing a wider, yet sparse exteroceptive information, which has never been encountered during training.

\subsection{Details of hierarchical memory}\label{supp:hierarchical_memory}
The closest approach to our hierarchical memory approach is the neural scene representation method~\cite{hoeller2022neural}, where the robot's local map is reconstructed by introducing an autoregressive structure for predicting and generating the 3D reconstruction of the local map. The neural scene representation network receives the robot frame's transformation from a separate odometry module, current measured points, and previous 3D reconstruction. The key difference in our method is that we employed autoregression solely for explicit estimation of the $SE(3)$ transformation of the body frame of the robot over time. Our proposed method does not require a complex reconstruction method with high capacity network, but still able to provide a temporally dense exteroception.

This estimated transformation is then utilized to transform the last observed points into the robot's current frame. The $SE(3)$ transformation is available at each control loop iteration via the state estimation network, enabling temporal interpolation of the latest exteroceptive measurements. This interpolation forms the basis of a memory structure, which is subsequently fed into the exteroceptive encoder. The exteroceptive observation is formally defined as

\begin{equation}
  \textbf{o}^{\mathrm{e},K}_t = \textbf{o}^\mathrm{e}_t \concat \hat{\textbf{o}}^\mathrm{e}_{t-1} \concat \cdots \concat \hat{\textbf{o}}^\mathrm{e}_{t-K}, 
\end{equation}
 where $\textbf{o}^\mathrm{e}_t$ is the most recent exteroceptive observation at time $t$. $\hat{\textbf{o}}^\mathrm{e}_{t-K}$ is the previous exteroceptive observation at $t-K$, which has been transformed to the robot's body frame at time $t$, which is defined as
\begin{equation}
  \hat{\textbf{o}}^\mathrm{e}_{t-K} = \prescript{t}{t-K}{T}^{-1}\cdot \textbf{o}^\mathrm{e}_{t-K},
\end{equation}
where $\textbf{o}^\mathrm{e}_{t-K}$ is the exteroceptive observation measured at time $t-K$, and $\prescript{t}{t-K}{T}$ is the $SE(3)$ transformation of the robot's pose from time $t$ to $t-K$. 
% 

% By doing so, our approach yields a lightweight architecture that retains some memory of the exteroceptions without necessitating memory-based networks.

\subsection{Scalability to other platforms}\label{supp:scalability}
We assessed the scalability of DreamWaQ++ with applications to legged robots with various morphologies and sizes. We used DreamWaQ++ to train a controller for an ANYmal-C~\cite{hutter2016anymal} and Hound~\cite{shin2022design} robots. Note that we used the same rewards and its corresponding weights as in supplementary section~\ref{supp:reward_functions} and only changed the robot's model as well as their motor's stiffness and damping parameter. A compilation of these robots navigating over stairs is provided in \mvseven. 

\figinitref{figure:supp_multi_robot} shows the success rates of three different robots on climbing stairs with various runs and rises. For the Go1 robot, we used a run value of $0.3~\mathrm{m}$ and $0.6~\mathrm{m}$, while for ANYmal-C and Hound, we used a run value of $0.6~\mathrm{m}$ and $1.0~\mathrm{m}$ to accommodate for their long trunk size. The success rates are measured from $1,\!000$ simulated robots, which is defined as the percentage of the number of robots that can reach the last stair within $10~\mathrm{s}$ over the total number of robots.
% , where a success is defined as when the robot can reach the last stairs within $10~\mathrm{s}$.

As expected, the large joint operation range of Hound enabled it to traverse more difficult terrains compared with the Go1 and ANYmal-C robot, allowing it to traverse up to $42~\mathrm{cm}$-high stairs with an $80\%$ success rate. It is also noteworthy that during training, the robots are faced only with a maximum obstacle height of $27~\mathrm{cm}$, and this result highlights the strong adaptability of the controller trained with DreamWaQ++. Thanks to the explorative behavior during training, DreamWaQ++ also maximizes the hardware's capability and the reward functions are invariant to the hardware variations.

\begin{figure}[t!]
	\centering 
	\begin{subfigure}[b]{0.48\textwidth}
		\includegraphics[width=1.0\textwidth]{figures/supp/supp_multirobot_success.pdf}
	\end{subfigure}
	% \captionsetup{font=footnotesize}
	\caption{\textbf{Success rates for climbing different obstacles using various quadrupedal robots.} We trained DreamWaQ++ for \textbf{(A)} Unitree Go1, \textbf{(B)} ANYmal-C, and \textbf{(C)} Hound. The maximum stair rise imposed during training for all robots is $27~\mathrm{cm}$.}
	\label{figure:supp_multi_robot}
\end{figure}

This evaluation successfully highlights the versatility of DreamWaQ++ for its applications to various legged robots. Although deep RL algorithms are notoriously sensitive to reward parameters for different robots, we discovered that DreamWaQ++ can be easily adopted to different platforms with no further tuning effort. 

\subsection{Learning to overcome large obstacles}\label{supp:parkour}
Recently, there has been a growing interest in training quadrupedal robots for more complex tasks such as jumping and leaping~\cite{hoeller2023anymal,zhuang2023robot}. These skills require the quadruped robot to maximize its actuator limit and orchestrate highly-agile motions. We further assessed the scalability of DreamWaQ++ in learning a skill required for overcoming obstacles that are higher than the robot. We trained the Go1, ANYmal-C, and Hound robots in an environment with extreme obstacle heights, reaching up to $0.6~\mathrm{m}$, $1.0~\mathrm{m}$, and $1.5~\mathrm{m}$, respectively. To allow learning of such an agile skill, we need to do some modifications, i.e., 1) relaxing the velocity tracking reward scale from $1.0$ to $0.1$, and 2) increasing the versatility gain scaling in the total loss function from $0.1$ to $0.2$. A snapshot of the learned obstacle climbing motion in simulation and the real world is shown in Fig.~\ref{figure:supp_parkour_sim} and \\mveight.

We found that the two modifications are complimentary. Relaxing the velocity tracking reward without scaling up the versatility gain ends up with a policy that resists moving forward. On the other hand, doubling the versatility gain without relaxing the velocity tracking reward results in a policy that moves forward but with a conservative gait due to lack of skill discovery. This modification allowed the policy to learn more flexible gaits, yielding higher agility for accomplishing more complex tasks such as parkour.

\begin{figure}[t!]
	\centering 
	\begin{subfigure}[b]{0.48\textwidth}
		\includegraphics[width=1.0\textwidth]{figures/supp/supp_parkour_sim_red.pdf}
	\end{subfigure}
	% \captionsetup{font=footnotesize}
	\caption{\textbf{Demonstration of a learned parkour skills in simulation.} We trained DreamWaQ++ for \textbf{(A)}~Unitree Go1, \textbf{(B)}~ANYmal-C, and \textbf{(C)}~Hound to climb obstacles with a height of $0.6~\mathrm{m}$, $1.0~\mathrm{m}$, $1.5~\mathrm{m}$, respectively. \textbf{(D)}~A real world experiment was conducted using a Go1 robot with a $2.5~\mathrm{kg}$ payload on top of it.}
	\label{figure:supp_parkour_sim}
\end{figure}

The results in Fig.~\ref{figure:supp_parkour_sim} illustrate how controllers on different robots produce distinct motions when overcoming large obstacles. In Fig.~\ref{figure:supp_parkour_sim}A, Go1 utilizes a jumping motion to overcome the obstacle, given its small posture. In contrast, ANYmal-C employs its front legs to establish initial contacts with the wall of the obstacle (Fig.~\ref{figure:supp_parkour_sim}B-2) and then uses those legs as anchors to climb (Fig.~\ref{figure:supp_parkour_sim}B-3). Thanks to its large allowable joint positions and torque operation limits, ANYmal-C can climb obstacles as high as $1.5~\mathrm{m}$. Hound, on the other hand, firstly swings its right front leg widely and places it on top of the obstacle as an anchor. Subsequently, it uses its rear legs to propel its body upward (Fig.~\ref{figure:supp_parkour_sim}C-4) and successfully reaches the top of the obstacles.

The real-world experiment in Fig.~\ref{figure:supp_parkour_sim}D was conducted to validate the sim-to-real robustness of the learned controller. Utilizing a Go1 robot with an additional $2.5\mathrm{kg}$ payload, the controller successfully enables the robot to climb a $41~\mathrm{cm}$ obstacle. Notably, the obstacle is a soft sofa block, representing a deformable surface not encountered during training.

% \subsection{Extreme terrain retraining}\label{supp:extreme}
% We further evaluate the versatility of DreamWaQ++ in a more challenging training setting. We fine-tuned the learned controller in a new training setting, consisting of extremely challenging terrains that can push the limit of the robot's physical capabilities, such as large gaps and high stages.

\subsection{Ablation of backbone sequence model}\label{supp:model_ablation}
We conducted an ablation study to evaluate the impact of the backbone sequence model on the controller's performance. We compared the performance of the controller with and with different sequence models by measuring the accuracy of future joint position prediction. The results are shown in Fig.~\ref{figure:supp_nextstate}.

\begin{figure}[t!]
	\centering 
	\begin{subfigure}[b]{0.48\textwidth}
		\includegraphics[width=1.0\textwidth]{figures/supp/supp_nextstate_red.pdf}
	\end{subfigure}
	% \captionsetup{font=footnotesize}
	\caption{\textbf{Future state error comparison.} The comparison shows the future state prediction error using different models and varying robot velocities.}
	\label{figure:supp_nextstate}
\end{figure}

The results in Fig.~\ref{figure:supp_nextstate} show that the proposed MLP-mixer architecture model works as well as the Transformer model. The advantage of using the MLP mixer is that it is more lightweight and computationally efficient than the Transformer model. From the curve, we can see that the prediction error increases as the robot's velocity increases. This is because the robot's motion becomes more dynamic and the model has to predict the future state more accurately.

\subsection{Terrain reconstruction}\label{supp:recons}
We decoded the latent features from the context encoder recorded in the asynchronous stair race experiment to reconstruct the terrain map. The reconstructed terrain map is shown in Fig.~\ref{figure:supp_recons} and \mvone0. The reconstructed terrain map resembles the ground truth terrain map constructed using~\cite{oh2024trip}.

However, note that the reconstructed terrain map is not as accurate as the ground truth terrain map due to three reasons: 
\begin{enumerate}
	\item The robot's exteroception is limited to the front-facing 3D points, and the memory retained by the encoder is not a long term memory.
	\item The encoder-decoder structure does not use a residual connection, similar to~\cite{hoeller2023anymal} to allow learning of only relevant features to the latent representation.
	\item The regularization in the latent space using a variational autoencoder is expected to reduce the reconstruction accuracy while improving disentanglement of the latent features. 
\end{enumerate}
Nevertheless, a slight reduction in the reconstruction accuracy is acceptable because the primary goal of the context encoder is to learn a structured representation that can be used for control, rather than to reconstruct the complete terrain map accurately.

\begin{figure}[t!]
	\centering 
	\begin{subfigure}[b]{0.48\textwidth}
		\includegraphics[width=1.0\textwidth]{figures/supp/supp_recons_red.pdf}
	\end{subfigure}
	% \captionsetup{font=footnotesize}
	\caption{\textbf{Reconstructed terrain map.} The terrain map is reconstructed from the latent features recorded during the asynchronous stair race using DreamWaQ++. The ground truth terrain map is constructed using~\cite{oh2024trip}. The white points are the forward 3D scan input, while the reconstruction points surrounding the robots are colored based on the height relative to the robot's base.}
	\label{figure:supp_recons}
\end{figure}
